# Supplementary material for: New Metrics to Evaluate the Performance and Fairness of Personalized Federated Learning
Source: arXiv:2107.13173 source file (2021-07-28)
Supplement: Supplementary file 1 [file appendix.tex]

% \documentclass{article}

% Recommended, but optional, packages for figures and better typesetting:
% \usepackage{microtype}
% \usepackage{graphicx}
% \usepackage{subfigure}
% \usepackage{booktabs} % for professional tables

% hyperref makes hyperlinks in the resulting PDF.
% If your build breaks (sometimes temporarily if a hyperlink spans a page)  berkay test
% please comment out the following usepackage line and replace
% \usepackage{icml2021} with \usepackage[nohyperref]{icml2021} above.
% \usepackage{hyperref}

% Attempt to make hyperref and algorithmic work together better:

% Use the following line for the initial blind version submitted for review:
% \usepackage{icml2021}

% If accepted, instead use the following line for the camera-ready submission:
%\usepackage[accepted]{icml2021}

% The \icmltitle you define below is probably too long as a header.
% Therefore, a short form for the running title is supplied here:
\icmltitlerunning{Alternative Metrics for the Evaluation of Personalized Federated Learning}

% \begin{document}

\appendix
\section{Appendix}

% The mapping between the numbers present in the Dataset Name column of Table~\ref{table:relatedWorks}, are mapped to the actual names of the datasets in Table~\ref{tab:datasetNames_Mapper}.

% % Dataset name mapping table.
% \input{tables/datasetNames_Mapper}
