# Supplementary material for: New Metrics to Evaluate the Performance and Fairness of Personalized Federated Learning
Source: arXiv:2107.13173 source file (2021-07-28)
Supplement: Supplementary file 2 [file appendix.tex]

% \documentclass{article}

% % Recommended, but optional, packages for figures and better typesetting:
% \usepackage{microtype}
% \usepackage{graphicx}
% \usepackage{subfigure}
% \usepackage{booktabs} % for professional tables

% % hyperref makes hyperlinks in the resulting PDF.
% % If your build breaks (sometimes temporarily if a hyperlink spans a page)  berkay test
% % please comment out the following usepackage line and replace
% % \usepackage{icml2021} with \usepackage[nohyperref]{icml2021} above.
% \usepackage{hyperref}

% % Attempt to make hyperref and algorithmic work together better:
% \newcommand{\theHalgorithm}{\arabic{algorithm}}

% % Use the following line for the initial blind version submitted for review:
% \usepackage{icml2021}

% If accepted, instead use the following line for the camera-ready submission:
%\usepackage[accepted]{icml2021}

% The \icmltitle you define below is probably too long as a header.
% Therefore, a short form for the running title is supplied here:
\icmltitlerunning{New Metrics for Evaluation of Personalized Federated Learning Techniques}

% \begin{document}

\appendix
\section{Appendix}

% % Data Generator Module.

% % Sub-subsection.
% \subsection{Datasets}
% \label{datasets_supported}

% We currently support the CIFAR-10 and MNIST datasets, widely used in \texttt{FL} training in the literature.
% %Still, it is straightforward to use other datasets.
% %
% MNIST is a dataset of $\mathtt{28 \times 28}$ images of handwritten digits from $\mathtt{0}$-$\mathtt{9}$ consisting of $\mathtt{10}$ labels and $\mathtt{70,000}$ instances. CIFAR-10 is a dataset of $\mathtt{32 \times 32}$ color images with $\mathtt{10}$ classes and $\mathtt{60,000}$ instances. 
% %
% Other well-known datasets such as CIFAR-100 and Imagenet, and custom datasets can be easily integrated to the framework.

% %\berkay{what about model architectures?}
% %\sid{Will include it under Federated Model Generation section. Also we won't be able to explain the architectures in detail, so I'll just cite the relevant paper which use those architecture(s).}

% % Sub-subsection.
% \subsection{Data-splitting Strategies}
% \label{datasplits_supported}

% The data splitting module supports the following four different data-splitting techniques.
% %from the literature, detailed as follows. We plan to support other data-splits as well in the future.

% In data-split 1 (\textbf{DS-1}), each user has the same total number of samples but may have different classes and a different number of samples per class.
% %
% The statistical heterogeneity is varied by controlling the parameter $\mathtt{k}$, which controls the number of overlapping classes between each user. 
% %
% For example, $\mathtt{k=4}$ corresponds to a highly non-identical data partition, whereas $\mathtt{k=10}$ corresponds to a highly identical data partition across the participating users. In our experiments, we set $\mathtt{k}$ to 4 to have non-IID data across users. 

% %
% In \textbf{DS-2}, all users have samples from all classes, but the number of samples per class they have is different, and hence the total number of samples per user is also different across users. 
% %
% %(Independent \& Identically Distributed)
% In order to simulate a non-IID distribution, we assign samples from each class to the users using a Dirichlet distribution with $\mathtt{\alpha = 0.9}$, following the previous work~\cite{nIID_dist}. Each class is parameterized by a vector $\mathtt{q}$ where $\mathtt{q \geq 0, i \in [1, N]}$, where $\mathtt{q}$ is sampled from a Dirichlet distribution with parameters $\mathtt{\alpha}$ and $\mathtt{p}$. 
% %
% The parameter $\mathtt{p}$ is the prior class distribution over the classes, and $\mathtt{\alpha}$ is the concentration parameter that controls the data similarity among the users. 
% %
% If $\mathtt{\alpha \rightarrow \infty}$, all users have an identical distribution to the prior. If $\mathtt{\alpha \rightarrow 0}$, each user only has samples from one class randomly chosen. 

% For \textbf{DS-3}, each user has two of the ten class-labels. 
% %
% Additionally, the total number of samples per user is different, \ie all the users do not have the same number of total samples. 
% %
% The samples assigned to users are drawn from a log-normal distribution with the parameters $\mathtt{\mu = 0}$ and $\mathtt{\sigma = 2}$.
% %
% A variable $\mathtt{u}$ has a log-normal distribution if $\mathtt{log(u)}$ is normally distributed. 
% %
% The probability density function for the log-normal distribution is computed as:

% \begin{equation}
%     \mathtt{p(u) = \frac{1}{\sigma u \sqrt{(2\pi)}} e^{-(\frac{(ln(u) - \mu)^2}{2\sigma^{2}})}}
%     \label{eqn:eqn_2}    
% \end{equation}

% These parameters correspond to the underlying normal distribution from which we draw the samples.

% % Describe the sampling process for DS-4.
% \textbf{DS-4} is introduced in \texttt{Per-FedAvg}~\cite{metaFL_2}. In this technique, assuming there are $\mathtt{n}$ users, then the data is split as follows. Half of the users ($\mathtt{\frac{n}{2}}$), have $\mathtt{k}$ images of each of the first five classes, and the remaining users ($\mathtt{\frac{n}{2}}$), have $\mathtt{\frac{k}{2}}$ images from only \textit{one} of the first five classes and $\mathtt{2k}$ images from only \textit{one} of the remaining five classes. The parameter $\mathtt{k}$ is set as $\mathtt{k = 196}$ and $\mathtt{k = 68}$ for MNIST, and CIFAR-10 respectively.

% % Federated Model Generation Module.
% \subsection{Model Architectures}
% \label{subsec:modelArchitectures}

% Currently, we support the following model architectures commonly used in the literature. 
% %
% For the CIFAR-10 dataset, we use a CNN-based model with two 2-D convolutional layers separated by a MaxPool layer between them and followed by three fully connected (FC) layers.  
% %
% The fully connected layers have $400$, $120$, and $84$ hidden neurons. We use ReLu activations after each layer except the last FC layer.
% %
% For the MNIST dataset, we use a two-layer deep neural network (DNN) with $100$ hidden-layer neurons, with a ReLu activation on the hidden layer. 
% %
% The output layer has $10$ nodes with a softmax function to get the class probabilities. The architectures we use for both datasets are similar to those in \texttt{pFedMe} for conformity.
% % 
% Extensions to support other architectures is straightforward.

% % Evaluation Metrics Section
% \subsection{Generalization of Metrics to FL} 

% The evaluation metrics introduced in this section are not restricted to personalized \texttt{FL}. They can also be applied in the \texttt{FL} setting. 
% %
% There have been diverse federated optimizers proposed in \texttt{FL} as an alternative to the base \texttt{FedAvg}, such as \texttt{FedBoost}~\cite{fedBoost}, \texttt{STC}~\cite{stc}, \texttt{FedAT}~\cite{fedAT}, \texttt{Overlap-FedAvg}~\cite{overlap_FL}.

% In these works, a new optimizer's performance is compared against \texttt{FedAvg} and other \texttt{FL} algorithms using only average accuracy.
% %
% The evaluation metrics introduced for personalized \texttt{FL} approaches can be used to evaluate the fairness across the users and measure the performance of federated optimizers other than solely reporting the average accuracy. 

% \begin{figure*}[hb!]
%     \centering 
%     \subfigure[\textbf{DS-2}]{\includegraphics[width=0.33\textwidth]{images/Density_2.png}} 
%     \subfigure[\textbf{DS-3}]{\includegraphics[width=0.33\textwidth]{images/Density_3.png}}
%     \caption{Density plots of \texttt{QoI} across \textbf{DS-2} and \textbf{DS-3} for CIFAR-10.}
%     \label{fig:densityPlots}
% \end{figure*}

% % CIFAR-10 Combined DS Fairness Metrics.
% \begin{figure*}[t!]
% \begin{center}
% \centerline{\includegraphics[width=2.1\columnwidth]{images/CIFAR10_Fairness_DS2&DS3.png}}
% \caption{Fairness metrics applied to the personalized algorithms on different data-splits of CIFAR-10. The first row is for \textbf{DS-2} and the second row is for \textbf{DS-3}.
% } 
% \label{fig:fairness_CIFAR10}
% \end{center}
% \end{figure*}

% % System Figure
% \begin{figure}[t!]
% \begin{center}
% \centerline{\includegraphics[width=1\columnwidth]{images/EvalFramework.pdf}}
% \caption{System Architecture}
% \label{fig:sysArch}
% \end{center}
% \end{figure}

% \end{document}
